# Supplementary material for: How to Teach Programming in the AI Era? Using LLMs as a Teachable Agent for Debugging
Source: arXiv:2310.05292 source file (2024-10-10)
Supplement: Supplementary file 1 [file appendix.tex]

\onecolumn
\section{LLM Prompts}
\label{appen:prompt}

\begin{table*}
\fontsize{7}{7.5}\selectfont
%\small
\begin{tabular}{R{0.07\textwidth} p{0.12\textwidth} | p{0.65\textwidth} | l | r}
\toprule
\materialtitle{Material} & \textbf{Generation goal} &
    \textbf{Model} & \textbf{T} \\

\arrayrulecolor{black!100}\midrule
\materialtitle{Test case category hint}
    & To generate test categories that are meaningful for the programming exercise.
    & GPT-3.5 & 0.3 \\
\arrayrulecolor{black!30}\midrule
%%%%%%%%%%%%%%%%%%%
\sysprompt{You are a helpful and experienced teaching assistant of an introductory programming class.}
\userprompt{Problem Description: \tinput{problem\_description}. List three most important aspects of this problem that need to be tested by describing the type of input. Write only each aspect in 3-6 words}
\llmprompt{\toutput{A list of test category names}}
%%%%%%%%%%%%%%%%%%%%

\arrayrulecolor{black!100}\midrule
\materialtitle{Test case desc. hint}
    & To accurately describe the key aspect a test case is covering.
    & GPT-3.5 & 0.1 \\
\arrayrulecolor{black!30}\midrule
%%%%%%%%%%%%%%%%%%%
\sysprompt{You are a helpful and experienced teaching assistant of an introductory programming class.}
\userprompt{Problem Description: \tinput{problem\_description}. Briefly describe this test case's input and explain what important aspect of this problem that the following test case covers: \tinput{test\_case}}
\llmprompt{\toutput{A description of the key aspect}}
\userprompt{Reformat it as a one-sentence hint. Use this template: Write a test case to cover the scenario where ...}
\llmprompt{\toutput{One sentence hint in the right format}}
%%%%%%%%%%%%%%%%%%%%

\arrayrulecolor{black!100}\midrule 
\materialtitle{Buggy code}
    & To over-generate bugs with mixed quality for selecting behaviorally distinct practice codes.
    & GPT-3.5 & 0.7 \\
\arrayrulecolor{black!30}\midrule
%%%%%%%%%%%%%%%%%%%
\sysprompt{You are a \textbf{novice student in intro CS}, you make mistakes and write buggy code when solving a problem.}
\userprompt{
\#\#\# Problem Description: \tinput{problem\_description} \newline
\#\#\# Instruction: Write \textbf{different buggy solutions} with common mistakes like novice students.\newline
\#\#\# Buggy Implementations:}
\llmprompt{\toutput{buggy code \#1}}
\llmprompt{\toutput{buggy code \#2}}
\llmprompt{\toutput{...}}
%%%%%%%%%%%%%%%%%%%%

\arrayrulecolor{black!100}\midrule
\materialtitle{Bug explanation and fix instruction}
    & To describe each unique bug, and write a corresponding fix instruction. If there are multiple bugs in the code, generate their explanations and fixes separately.
    & GPT-4 & 0.3 \\
\arrayrulecolor{black!30}\midrule
%%%%%%%%%%%%%%%%%%%
\sysprompt{You are a helpful and experienced \textbf{teaching assistant} of an introductory programming class.}
\userprompt{Hi, I'm a student in your class. I'm having trouble with this problem in the programming assignment: \tinput{problem\_description}  I've tried to fix my code but I'm still stuck. Can you help me?}
\llmprompt{Sure, let's take a look at your code.}
\userprompt{Here's my buggy code: \tinput{buggy\_code}
What's wrong with my code? \textbf{List all the unique bugs included, but do not make up bugs}. For each point, put in the format of: \{explanation: accurate and concise explanation of what the code does and what the bug is, for a novice, fix: how to fix the bug, within 30 words\} \newline 
Only \textbf{return the bullet list}. Do not write any other text or code.}
\llmprompt{\toutput{Bullet list of json formats with explanation and fixes}}
%%%%%%%%%%%%%%%%%%%%

\arrayrulecolor{black!100}\midrule
\materialtitle{Bug fix}
    & To edit the buggy code according to the fix instruction, without over- or under- fix.
    & GPT-3.5 & 0.3 \\
\arrayrulecolor{black!30}\midrule
%%%%%%%%%%%%%%%%%%%
\sysprompt{You fix bugs in Python code closely following the instructions.}
\userprompt{
Original code: \tinput{buggy\_code}; Code modification: \tinput{explanation} \newline
\textbf{Translate the statement into actual, minimal code change in this format}: \newline
\{original code snippet: ""copy the lines of code that need editing"" \newline -> edited code snippet: ""write the edited code snippet""\}}
\llmprompt{\toutput{JSON formatted old to new snippet, e.g., \texttt{\swap{numbers\_list[i] <= key}{numbers\_list[i] > key}} }}
\arrayrulecolor{black!0}\midrule
\sysprompt{You fix bugs in Python code closely following the instructions.}
\userprompt{
Old Code:\tinput{buggy\_code}; Instruction:\tinput{Old snippet to new snippet}; New Code:}
\llmprompt{\toutput{The complete version of the new fixed code}}

%%%%%%%%%%%%%%%%%%%%

\arrayrulecolor{black!100}\bottomrule

\end{tabular}

\caption{Parameters used for generating training materials: prompts, the LLM model used, and the corresponding temperature. }
\label{tab:prompt}
\vspace{-20pt}
\end{table*}

\section{LLM Experiment Materials}

\label{appen:exercise}
%%%%%%%%%%%%%%%%%% problems

% \cref{tab:problems} summarized the problem description, number of generated bugs, and number of final fixed codes for each of the six problems used in LLM experiment.
\lstset{
  basicstyle=\ttfamily, % Using a smaller font size for listings
  columns=fullflexible,
  breaklines=false,
  % postbreak=\mbox{\textcolor{red}{$\hookrightarrow$}\space},
  % tabsize=2, % Sets the tab size to 2 spaces
  % frame=single % Adds a frame around the code
}

\begin{table}[htb]
\small
\caption{Description, number of generated bugs, and number of final fixed codes for problems used in LLM experiment} %LLM experiment problem descriptions and statistics}
\label{tab:problems}
\begin{tabular}{p{0.2\textwidth} p{0.65\textwidth} r r}
\toprule
\textbf{Problem} & \textbf{Description} & \textbf{\# Bugs} & \textbf{\# Fixes} \\
\midrule 
first\_num\_greater\_than & 
\begin{lstlisting} 
Write a Python function first_num_greater_than(numbers_list, key) 
that takes a list of integers (numbers_list) and an integer key (key), 
and returns the first number in the list that is greater than the key.
If there is no number greater than the key, then you should return None.\end{lstlisting}
& 30 & 36 \\
\midrule
remove\_extras & 
% \begin{tabminted}{tea}
\begin{lstlisting}
Function remove_extras(lst) takes in a list of integers and returns 
a new list with the first occurrence of each element, which is the 
same as lst but with all repeated occurrences of any element removed.
\end{lstlisting} 
& 23 & 31 \\
\midrule
num\_smaller & 
\begin{lstlisting}
Function num_smaller(seq, x) takes in an integer x and a sorted 
integer sequence seq, and returns the number of elements in seq 
that is strictly smaller than x.
\end{lstlisting} 
& 18 & 24 \\
\midrule
sort\_age & 
\begin{lstlisting}
We represent a person using a tuple (<gender>, <age>). Given a list
of people, write a function sort_age that returns a list in an order
such that the older people are at the front of the list. You may 
assume that no two members in the list of people are of the same age.
\end{lstlisting}
& 28 & 42 \\
\midrule
top\_k & 
\begin{lstlisting}
Write a function top_k that takes a list of integers as the input 
and returns the greatest k number of values as a list, with its 
elements sorted in descending order. You may use any sorting algorithm, 
but you are not allowed to use the Python function sort and sorted.
\end{lstlisting}
& 28 & 42 \\
\midrule
swap\_keys\_values & 
\begin{lstlisting}
Write a function swap_keys_values that takes in a dictionary, and 
returns a new dictionary with the keys and values swapped.
\end{lstlisting}
& 18 & 20 \\
\midrule
\textbf{Total} &  &  145 & 195 \\
\bottomrule
\end{tabular}
\end{table}

More details in \cref{tab:metrics}.
\begin{itemize}[labelwidth=*,leftmargin=1.3em,align=left]

\item \emph{Test case category hint}:
A good test case category should be \emph{reasonable to test for a problem}. We define the success rate as the proportion of \emph{suitable test categories} over all the test categories per problem.

\item \emph{Test case description hint}: 
A good test case hint should accurately \emph{describe the test case behavior}.
We define the success rate as the proportion of test case hints that provide an accurate description.

\item \emph{Buggy codes}: 
Intuitively, we prefer buggy codes that add more meaningful variations to existing buggy code collections. 
Therefore, we define success rate as \emph{the ratio of behaviorally distinct codes}, where code behavior is automatically categorized with instructor-provided reference test inputs.

\item \emph{Bug explanation and fix instruction}:
As the prompt requires identifying multiple bugs, we manually evaluate each pair of explanation and fix instructions, and count one generation as correct when there is a matching explanation and the corresponding fix, and both are correct.\footnote{In some cases the LLM describes the same bug twice because there are conceptual differences between them even when they actually share the same fix. We still count this as correct, as they only require humans to delete the extra bugs.}

\item \emph{Bug fix}:
We define a bug fix to be a success if the \{ old code snippet $->$ new code snippet \} accurately reflects the instruction without over- or under- fix.

\end{itemize}

\begin{table*}[htb]
\small
\caption{Human annotation tasks and success rate definitions for each type of material generated in LLM experiment}
\label{tab:metrics}
\begin{tabular}{p{0.14\textwidth} p{0.19\textwidth} p{0.58\textwidth} }
\toprule
\textbf{Material}  & \textbf{Success Rate Definition} & \textbf{Human Label Tasks}  \\
\midrule
Buggy code & 
\multirow{2}{*}{$\frac{\text{\# behaviorally distinct buggy code }}{\text{ \# non-identical buggy code }}$} & 
remove extra comments %  \mint{python}| (e.g., # the operator should actually be >)| % spacing is off
% \begin{tabminted}{python}

\lstinline|e.g., # the operator should actually be >|
\\
\midrule
Bug explanation and fix instruction & 
\multirow{4}{*}{$\frac{\text{\# correct expl \& fix }}{\text{ \# total buggy code }}$}
& \texttt{multibug\_correct: T/F} (does this code have meaningful and isolate fixes specify for the bug(s) listed), \texttt{NA} (there is only one single bug as specified) \\
& & \texttt{expl\_correct: T/F} (does the explanation accurately reflect the bug in code) \\
& & \texttt{fix\_correct: T/F} (does the fix correctly and minimally fix the bug in code) \\
& & \texttt{edited\_expl\_fix:} edited for next step if needed \texttt{\{expl:...; fix:...\}} \\
\midrule
Fixed Code &
\multirow{3}{*}{$\frac{\text{\# accurately fixed code }}{\text{ \# total buggy code }}$}
& \texttt{fix\_round1\_correct: T/F} (does the code snippet accurately reflect the instruction without over- or under-fix) \& \texttt{edited\_round1\_fix:} edited fix lines if needed \\
& & \texttt{fix\_round2\_correct: T/F} (does the fixed code accurately reflect the instruction without over or under-fix) \& \texttt{edited\_fixed\_code:} edited fix code if needed \\
\midrule
Test case description hint & 
\multirow{2}{*}{$\frac{\text{\# correct test case hint }}{\text{ \# total test case }}$} & 
\texttt{tc\_hint\_correct: T/F} (does this hint accurately describe what the test case is doing) \& \texttt{edited\_tc\_hint:} edited test case hint if needed \\
\midrule
Test case category & 
\multirow{2}{*}{$\frac{\text{\# correct test category }}{\text{ \# total test category }}$} & 
\texttt{tc\_category\_correct: T/F} (is this category reasonable to test for this problem) \& \texttt{edited\_tc\_category:} edited category if needed \\
\bottomrule
\end{tabular}
\end{table*}
